# Supplementary material for: Sensitivity of BPA SAR Image Formation to Initial Position, Velocity, and Attitude Navigation Errors
Source: arXiv:2009.10210 source file (2020-09-21)
Supplement: Supplementary file 1 [file nav-appendix.tex]

This appendix derives the error state differential equation \ref{eq:cov-err-state-diffeq},
by expanding the each term of the truth model in equation \ref{eq:cov-veh2}
about the estimated quantities in equations \ref{eq:cov-calcEstErrors1}
to \ref{eq:cov-calcEstErrors3}. Expansion of the position differential
equation yields
\begin{equation}
\dot{\hat{\boldsymbol{p}}}^{n}+\delta\dot{\boldsymbol{p}}^{n}=\hat{\boldsymbol{v}}^{n}+\delta\boldsymbol{v}^{n}
\end{equation}
Subtraction of the navigation dynamics in equation \ref{eq:cov-veh7}
yields the error state dynamics for position
\begin{equation}
\delta\dot{\boldsymbol{p}}^{n}=\delta\boldsymbol{v}^{n}\label{eq:app-poserr}
\end{equation}

After substitution of the accelerometer measurement model in equation
\ref{eq:cov-cont-inertial-measurements}, expansion of the truth velocity
differential equation and yields
\begin{equation}
\dot{\hat{\boldsymbol{v}}}^{n}+\delta\dot{\boldsymbol{v}}^{n}=\left[I-\left(\delta\boldsymbol{\theta}{}^{n}\times\right)\right]\hat{T}_{b}^{n}\left(\tilde{\boldsymbol{\nu}}^{b}-\boldsymbol{n}_{\nu}\right)+\boldsymbol{g}^{n}
\end{equation}
Subtraction of the navigation velocity dynamics in equation \ref{eq:cov-veh7}
and discarding second order terms yields
\begin{equation}
\delta\dot{\boldsymbol{v}}^{n}=-\left(\delta\boldsymbol{\theta}{}^{n}\times\right)\hat{T}_{b}^{n}\tilde{\boldsymbol{\nu}}^{b}-\hat{T}_{b}^{n}\boldsymbol{n}_{\nu}
\end{equation}
Reversing the cross product to move the attitude term to the right
yields the final form of the velocity error dynamics
\begin{equation}
\delta\dot{\boldsymbol{v}}^{n}=\left(\hat{T}_{b}^{n}\tilde{\boldsymbol{\nu}}^{b}\right)\times\delta\boldsymbol{\theta}{}^{n}-\hat{T}_{b}^{n}\boldsymbol{n}_{\nu}\label{eq:app-velerr}
\end{equation}

Lastly, the truth quaternion dynamics is expanded to yield
\begin{equation}
\dot{q}_{b}^{n}=\frac{1}{2}q_{b}^{n}\otimes\left[\begin{array}{c}
0\\
\boldsymbol{\omega}^{b}\left(t\right)
\end{array}\right]
\end{equation}

Taking the derivative of \ref{eq:cov-calcEstErrors3} yields
\begin{equation}
\left[\begin{array}{c}
0\\
-\frac{1}{2}\delta\dot{\boldsymbol{\theta}}{}^{n}
\end{array}\right]=\dot{q}_{b}^{n}\otimes\left(\hat{q}_{b}^{n}\right)^{*}+q_{b}^{n}\otimes\left(\dot{\hat{q}}_{b}^{n}\right)^{*}
\end{equation}
Substitution of the truth and navigation quaternion kinematics yields
\begin{align}
\left[\begin{array}{c}
0\\
-\frac{1}{2}\delta\dot{\boldsymbol{\theta}}{}^{n}
\end{array}\right] & =\frac{1}{2}q_{b}^{n}\otimes\left[\begin{array}{c}
0\\
\boldsymbol{\omega}^{b}
\end{array}\right]\otimes\left(\hat{q}_{b}^{n}\right)^{*}\\
+ & q_{b}^{n}\otimes\left(\frac{1}{2}\hat{q}_{b}^{n}\otimes\left[\begin{array}{c}
0\\
\tilde{\boldsymbol{\omega}}^{b}
\end{array}\right]\right)^{*}
\end{align}
which is rearranged to become
\begin{equation}
\left[\begin{array}{c}
0\\
-\frac{1}{2}\delta\dot{\boldsymbol{\theta}}{}^{n}
\end{array}\right]=\frac{1}{2}q_{b}^{n}\otimes\left[\begin{array}{c}
0\\
\boldsymbol{\omega}^{b}-\tilde{\boldsymbol{\omega}}^{b}
\end{array}\right]\otimes\hat{q}_{n}^{b}
\end{equation}
Substitution of the angular rate error in equation \ref{eq:cov-cont-inertial-measurements}
yields
\begin{equation}
\left[\begin{array}{c}
0\\
-\frac{1}{2}\delta\dot{\boldsymbol{\theta}}{}^{n}
\end{array}\right]=\frac{1}{2}q_{b}^{n}\otimes\left[\begin{array}{c}
0\\
-\boldsymbol{n}_{\omega}
\end{array}\right]\otimes\hat{q}_{n}^{b}
\end{equation}
Expansion of the $q_{b}^{n}$ using equation \ref{eq:cov-calcEstErrors3}
yields
\begin{equation}
\left[\begin{array}{c}
0\\
-\frac{1}{2}\delta\dot{\boldsymbol{\theta}}{}^{n}
\end{array}\right]=\frac{1}{2}\left[\begin{array}{c}
1\\
-\frac{1}{2}\delta\boldsymbol{\theta}{}^{n}
\end{array}\right]\otimes\hat{q}_{b}^{n}\otimes\left[\begin{array}{c}
0\\
-\boldsymbol{n}_{\omega}
\end{array}\right]\otimes\hat{q}_{n}^{b}
\end{equation}
where it is noted that last three terms correspond to a transformation
of $\boldsymbol{n}_{\omega}$(see \cite{savage_strapdown_2000}, section
3.2.4.1)
\begin{equation}
\left[\begin{array}{c}
0\\
-\frac{1}{2}\delta\dot{\boldsymbol{\theta}}{}^{n}
\end{array}\right]=\frac{1}{2}\left[\begin{array}{c}
1\\
-\frac{1}{2}\delta\boldsymbol{\theta}{}^{n}
\end{array}\right]\otimes\left[\begin{array}{c}
0\\
-\hat{T}_{b}^{n}\boldsymbol{n}_{\omega}
\end{array}\right]
\end{equation}
Evaluation of the quaternion product yields

\begin{equation}
\left[\begin{array}{c}
0\\
-\frac{1}{2}\delta\dot{\boldsymbol{\theta}}{}^{n}
\end{array}\right]=\frac{1}{2}\left[\begin{array}{c}
\frac{1}{2}\delta\boldsymbol{\theta}{}^{n}\cdot\hat{T}_{b}^{n}\boldsymbol{n}_{\omega}\\
-\hat{T}_{b}^{n}\boldsymbol{n}_{\omega}-\frac{1}{2}\delta\boldsymbol{\theta}{}^{n}\times\hat{T}_{b}^{n}\boldsymbol{n}_{\omega}
\end{array}\right]
\end{equation}
Neglecting products of errors yields
\begin{equation}
\left[\begin{array}{c}
0\\
-\frac{1}{2}\delta\dot{\boldsymbol{\theta}}{}^{n}
\end{array}\right]=\frac{1}{2}\left[\begin{array}{c}
0\\
-\hat{T}_{b}^{n}\boldsymbol{n}_{\omega}
\end{array}\right]
\end{equation}
Equating the vector components provides the final result
\begin{equation}
\delta\dot{\boldsymbol{\theta}}{}^{n}=\hat{T}_{b}^{n}\boldsymbol{n}_{\omega}\label{eq:app-therr}
\end{equation}
